# Supplementary material for: Reverse Transition Kernel: A Flexible Framework to Accelerate Diffusion Inference
Source: arXiv:2405.16387 source file (2024-05-26)
Supplement: Supplementary file 1 [file emperical_notes.tex]

\section{Some notes about experiments}
In this section, we use notations shown in Section~\ref{sec:not_ass_app}.
We compare our methods with different inference algorithms, e.g., DDPM~(\cite{ho2020denoising}), DDIM~(\cite{song2020denoising}) and DPM-solver~(\cite{lu2022dpm}), from an empirical perspective.
\paragraph{Compared with DDPM.} 
Currently, most practical stable diffusion models are trained based on the formulation given in DDPM~(\cite{ho2020denoising}).
While in analysis, most theoretical frameworks are based on the reverse OU process. 
However, there is existing a scaling gap between the forward process of DDPM and the standard OU process.
Such a scaling gap may affect the derivation of our RTKI.
Hence, we denote the gap here.

We couple these two processes by investigating their training losses.
We first consider the standard OU process, i.e.,
\begin{equation*}
    \der \rvx_t = -\rvx_t \der t + \sqrt{2}\der \mB_t
\end{equation*}
whose closed-form satisfies
\begin{equation}
    \label{sde:ou_process}
    \begin{aligned}
        \rvx_t =  & e^{-t}\cdot \rvx_0  + \sqrt{2}\int_0^t  e^{-(t-s)} \der\mB_s= e^{-t}\cdot \rvx_0 + \sqrt{1-e^{-2t}}\xi\quad \mathrm{where}\quad \xi\sim \mathcal{N}(\vzero, \mI).
    \end{aligned}
\end{equation}
Moreover, the reverse OU process is 
\begin{equation*}
    \der \rbkwx_t = \left(\rbkwx_t + 2\grad\ln p_{T-t}(\rbkwx_t)\right)\der t +\sqrt{2} \der B_t.
\end{equation*}
The objective loss to parameterize the score function $\grad\ln p_{t}(\cdot)$ with neural nets $s_{\theta}(\cdot, t)$ will be
\begin{equation*}
    \min_{\theta}\ \E_{\rvx\sim p_t}\left[\left\|\grad \ln p_{t}(\rvx) - s_{\theta}(\rvx, t)\right\|^2\right]
\end{equation*}
According to Section A of~\cite{chen2022sampling}, the above objective loss can be reformulated as
\begin{equation}
    \label{def:rev_ou_loss}
    \E_{\rvx\sim p_t}\left[\left\|\grad \ln p_{t}(\rvx) - s_{\theta}(\rvx, t)\right\|^2\right] =  \E\left[\left\|s_{\theta}(\rvx_t,t) + \frac{1}{\sqrt{1-e^{-2t}}}\cdot \xi\right\|^2\right]
\end{equation}
where $\rvx_0\sim p_0$ and $\xi\sim \mathcal{N}(\vzero,\mI)$ are independent, and $\rvx_t$ follows from Eq.~\ref{sde:ou_process}.
Consider a discrete version, where we set $t=k\eta$, the objective loss will become
\begin{equation}
    \label{def:rev_ou_dis_loss}
      \E\left[\left\|s_{\theta}\left(\sqrt{e^{-2k\eta}}\rvx_0 + \sqrt{1-e^{-2k\eta}}\xi,k\eta\right) + \frac{1}{\sqrt{1-e^{-2k\eta}}}\cdot \xi\right\|^2\right],
\end{equation}
which intuitively means
\begin{equation}
    \label{approx:score_xi}
    -\sqrt{1-e^{-2k\eta}} \cdot s_{\theta}\left(\sqrt{e^{-2k\eta}}\rvx_0 + \sqrt{1-e^{-2k\eta}}\xi,k\eta\right) \approx \xi
\end{equation}
with a little abuse of notations.
When we check the training loss of DDPM, i.e., Eq.~(14) of~\cite{ho2020denoising}, it is nearly
\begin{equation}
    \label{def:ddpm_loss}
    \E\left[\left\|\tilde{s}_{\theta}(\sqrt{\overline{\alpha}_k}\rvx_0 + \sqrt{1-\overline{\alpha}_k}\xi, k) - \xi\right\|^2\right].
\end{equation}
If we choose
\begin{equation*}
    \overline{\alpha}_k = e^{-2k\eta}, \quad \alpha_k = e^{-2\eta}\quad \mathrm{and}\quad \beta_k = 1-\alpha_k = 1-e^{-2\eta}
\end{equation*}
where the definition of $\alpha_k$ and $\beta_k$ follows from the definition shown in~\cite{ho2020denoising}, we intuitively have
\begin{equation*}
    \tilde{s}_{\theta}\left(\sqrt{e^{-2k\eta}}\rvx_0 + \sqrt{1-e^{-2k\eta}}\xi,k\right)\approx \xi.
\end{equation*}
Compared with Eq.~\ref{approx:score_xi}, we may consider 
\begin{equation*}
\underbrace{\tilde{s}_{\theta}\left(\cdot,k\right)}_{\text{the output of neural nets at }k\eta} \approx -\sqrt{1-e^{-2k\eta}} \cdot \underbrace{s_{\theta}\left(\cdot,k\eta\right)}_{\approx \grad\ln p_{k\eta}(\cdot)}.
\end{equation*}

A deterministic scaling will help us to compare the inference differences between discretized reverse OU and DDPM. 
In the following, we denote $K\eta = T$ as the forward time.
For a discretized reverse OU, we consider the following SDE at the $k$-th step, i.e.,
\begin{equation}
    \label{sde:dr_OU}
    \der \rbkwx_t = \left(\rbkwx_t + 2 s_{\theta}(\rbkwx_{k\eta}, (K-k)\eta)\right)\der t +\sqrt{2} \der B_t,\quad\mathrm{where}\quad t\in(k\eta,(k+1)\eta] 
\end{equation}
whose closed solution satisfies
\begin{equation*}
    \rbkwx_{(k+1)\eta} =  \frac{1}{\sqrt{e^{-2\eta}}}\cdot\left[\rbkwx_{k\eta} + \frac{e^{\eta}-1}{e^{\eta}}\cdot 2s_{\theta}\left(\rbkwx_{k\eta},(K-k)\eta\right)\right] + \sqrt{e^{2\eta}-1}\cdot \xi.
\end{equation*}
According to~\cite{ho2020denoising}, the inference process of DDPM is 
\begin{equation*}
    \begin{aligned}
        \hat{\rvx}^\gets_{k+1} = & \frac{1}{\sqrt{\alpha_{K-k}}}\cdot \left[\hat{\rvx}^\gets_{k} - \frac{\beta_{K-k}}{\sqrt{1-\overline{\alpha}_{K-k}}}\cdot \tilde{s}_{\theta}\left(\hat{\rvx}^\gets_k, (K-k)\right)\right] + \sqrt{\beta_{K-k}}\cdot\xi\\
        = & \frac{1}{\sqrt{e^{-2\eta}}}\cdot \left[\hat{\rvx}^\gets_{k} + \frac{1-e^{-2\eta}}{2}\cdot \frac{-2\tilde{s}_{\theta}\left(\hat{\rvx}^\gets_k, (K-k)\right)}{\sqrt{1-e^{-2(K-k)\eta}}}\right] + \sqrt{1-e^{-2\eta}}\cdot\xi\\
        \approx & \frac{1}{\sqrt{e^{-2\eta}}}\cdot \left[\hat{\rvx}^\gets_{k} + \frac{1-e^{-2\eta}}{2}\cdot 2s_{\theta}(\hat{\rvx}_k^\gets, (K-k)\eta)\right] + \sqrt{1-e^{-2\eta}}\cdot\xi.
    \end{aligned}
\end{equation*}
Although the coefficients of $s_\theta(\cdot, (K-k)\eta)$ and $\xi$ are different, while they have the nearly the same growth when $\eta\rightarrow 0$, which can be found in Fig.~\ref{fig:rOU_ddpm_coe}.
Therefore, such two algorithms are nearly equivalent.
\begin{figure}
        \centering
        \includegraphics[width=10cm]{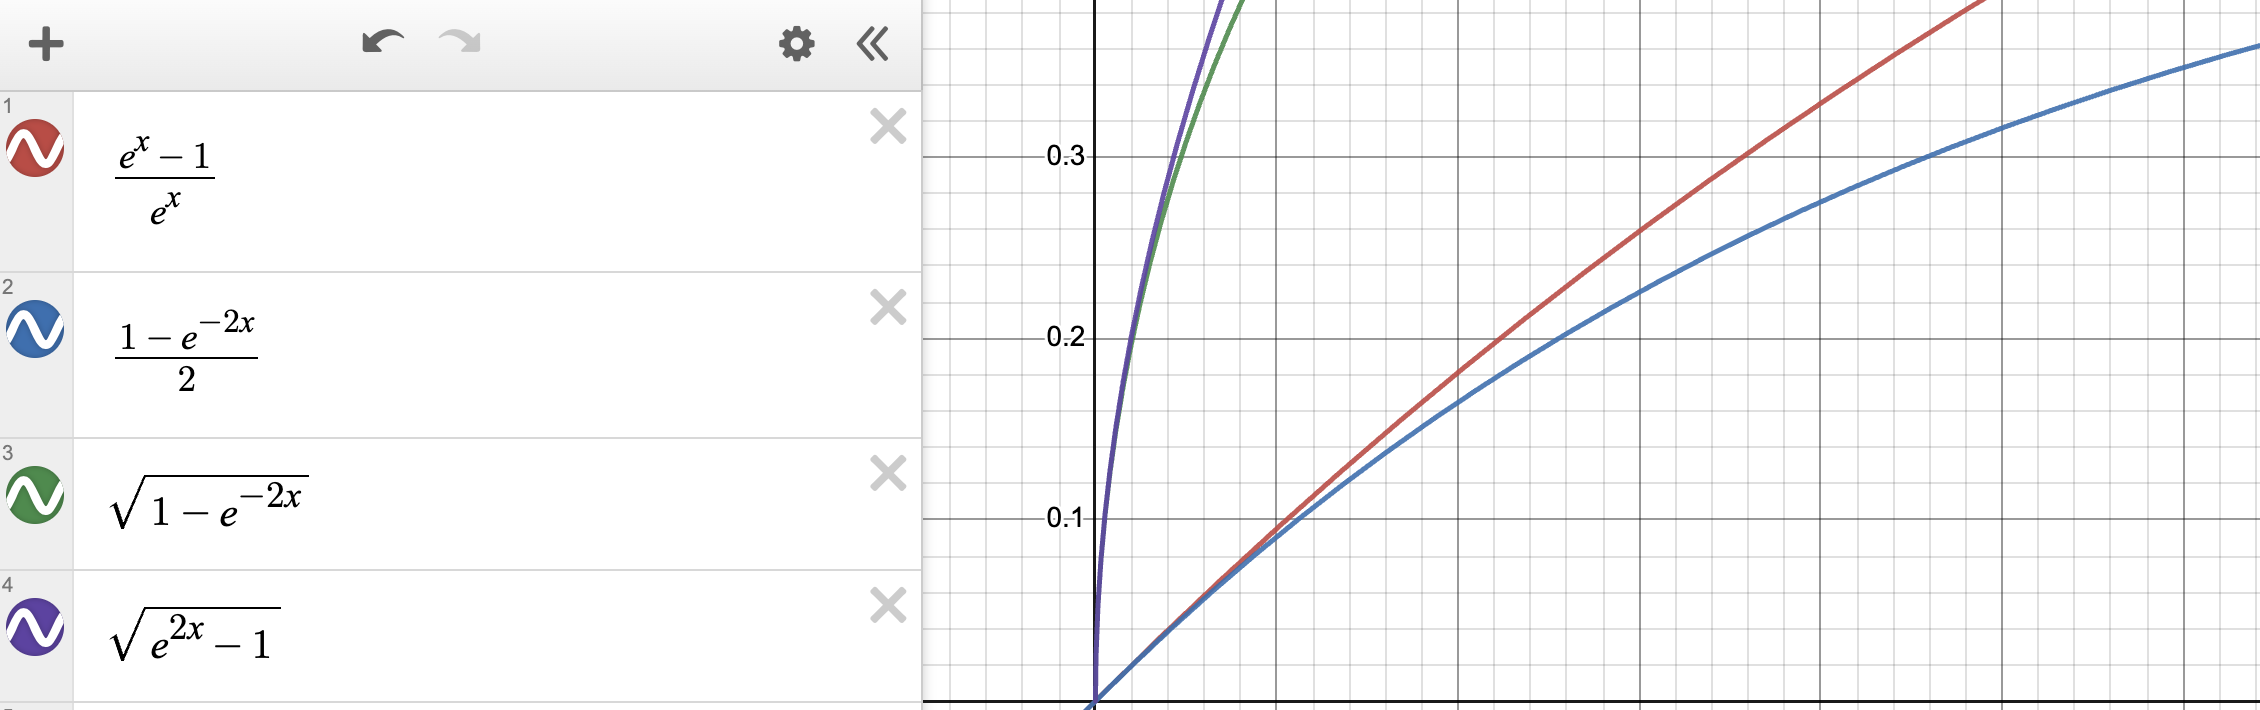}
        \caption{TBC}
        \label{fig:rOU_ddpm_coe}
\end{figure}
However, in real applications, DDPM is usually implemented in another way\footnote{\href{https://github.com/huggingface/diffusers/blob/v0.26.3/src/diffusers/schedulers/scheduling_ddpm.py}{DDPM Implementation in Diffusers}}, slightly different from Alg.2 shown in~\cite{ho2020denoising}.
Suppose $\overline{\beta}_k = 1-\overline{\alpha}_k$, it mainly has the following steps:
\begin{itemize}
    \item Construct an intermediate variable
    \begin{equation}
        \begin{aligned}
            \text{pred\_original\_sample} = & \frac{\hat{\rvx}^\gets_k - \sqrt{\overline{\beta}_{K-k}}\cdot \tilde{s}_{\theta}\left(\hat{\rvx}^\gets_k, (K-k)\right)}{\sqrt{\overline{\alpha}_{K-k}}}\\
            = & \frac{\hat{\rvx}_k^\gets}{\sqrt{\overline{\alpha}_{K-k}}} - \frac{\sqrt{1-\overline{\alpha}_{K-k}}\cdot \tilde{s}_{\theta}\left(\hat{\rvx}^\gets_k, (K-k)\right)}{\sqrt{\overline{\alpha}_{K-k}}}
        \end{aligned}
    \end{equation}
    \item Then, it has
    \begin{equation*}
        \begin{aligned}
            \text{pred\_prev\_sample} = & \frac{\sqrt{\overline{\alpha}_{K-(k+1)}}\cdot \beta_{K-k}}{\overline{\beta}_{K-k}}\cdot \text{pred\_original\_sample} + \frac{\sqrt{\alpha_{K-k}}\cdot \overline{\beta}_{K-(k+1)}}{\overline{\beta}_{K-k}}\cdot \hat{\rvx}_k^\gets\\
            = & \left(\frac{\sqrt{\overline{\alpha}_{K-(k+1)}}\cdot \beta_{K-k}}{\overline{\beta}_{K-k}}\cdot \frac{1}{\sqrt{\overline{\alpha}_{K-k}}}+ \frac{\sqrt{\alpha_{K-k}}\cdot \overline{\beta}_{K-(k+1)}}{\overline{\beta}_{K-k}} \right)\cdot \hat{\rvx}_k^\gets \\
            & - \frac{\sqrt{\overline{\alpha}_{K-(k+1)}}\cdot \beta_{K-k}}{\overline{\beta}_{K-k}}\cdot \frac{\sqrt{1-\overline{\alpha}_{K-k}}\cdot \tilde{s}_{\theta}\left(\hat{\rvx}^\gets_k, (K-k)\right)}{\sqrt{\overline{\alpha}_{K-k}}}\\
            = & \left(\frac{1-\alpha_{K-k}}{\sqrt{\alpha_{K-k}}\cdot (1-\overline{\alpha}_{K-k})} + \frac{\alpha_{K-k}\cdot (1-\overline{\alpha}_{K-(k+1)})}{\sqrt{\alpha_{K-k}}\cdot (1-\overline{\alpha}_{K-k})}\right)\cdot \hat{\rvx}_k^\gets\\
            & - \sqrt{\frac{\overline{\alpha}_{K-(k+1)}}{\overline{\alpha}_{K-k}}}\cdot \frac{\beta_{K-k}}{2}\cdot \frac{2\tilde{s}_{\theta}\left(\hat{\rvx}^\gets_k, (K-k)\right)}{\sqrt{1-\overline{\alpha}_{K-k}}}\\
            = & e^{\eta}\cdot \hat{\rvx}_k^\gets- e^{\eta}\cdot \frac{1-e^{-2\eta}}{2}\cdot 2s_{\theta}(\hat{\rvx}_k^\gets, (K-k)\eta)
        \end{aligned}
    \end{equation*}
    \item Add the noise, with scaling
    \begin{equation*}
        \frac{(1-\overline{\alpha}_{K-(k+1)})}{(1-\overline{\alpha}_{K-k})}\cdot \frac{(1-\overline{\alpha}_{K-k})}{\overline{\alpha}_{K-(k+1)}}\cdot \xi = \left(e^{2(K-k-1)\eta} - 1\right)\cdot \xi, 
    \end{equation*}
    which DOES NOT match the inference process of reverse OU and DDPM.
    This mistake may be from abuse of $\beta_k$ in~\cite{ho2020denoising}, which writes both conditional variances and total variance as $\beta_k$ both. 
    Actually, it should be conditional variance in iterations rather than the total variance.
\end{itemize}

\paragraph{Compared with DDIM.}
