# Supplementary material for: Reverse Transition Kernel: A Flexible Framework to Accelerate Diffusion Inference
Source: arXiv:2405.16387 source file (2024-05-26)
Supplement: Supplementary file 2 [file energy_estimation.tex]

% \section{Estimating the energy via score function }
% In the previous section, we assume that we can obtain an estimator for the energy function $f(\vx)$. However, in practice, we can only access the score network, which produces the estimation $s_{\theta}(\vx):=\nabla g(\vx)$ rather than $g(\vx)$. Therefore, in this part, we seek solutions for approximating the energy function using the score network $s_\theta(\vx)$. 

% In general, using the gradient to estimate the original energy function is intractable as we are missing the zero-th-order information. Fortunately, as shown in Algorithm \ref{alg:inner_mala}, we only need to tackle the difference between two energy functions, i.e., $r(\vx,\vx')=g(\vx) - g(\vx')$.  Therefore, the zero-th-order information of the energy function is canceled out and the first-order information is sufficient for estimation. 
