# Supplementary material for: Reverse Transition Kernel: A Flexible Framework to Accelerate Diffusion Inference
Source: arXiv:2405.16387 source file (2024-05-26)
Supplement: Supplementary file 3 [file backup.tex]

\section{Review of the inference of diffusion models}
Essentially, the inference of diffusion models can be considered as the discretization of the reverse OU process, i.e.,
\begin{equation}
    \label{sde:rev_ou}
    \der \rbkwx_{t} = \left(\rbkwx_t + 2 \grad \ln p_{T-t}(\rbkwx_t)\right) \der t + \sqrt{2}\der \mB_t
\end{equation}
where $p_t$ denotes the underlying distribution of $\rvx_t$ which satisfies
\begin{equation}
    \label{sde:ou}
    \der \rvx_t = -\rvx_t \der t + \sqrt{2}\der \mB_t \quad \mathrm{where}\quad \rvx_0\sim p_{\mathrm{data}}.
\end{equation}
To implement SDE.~\ref{sde:rev_ou} for inference, diffusion models parameterize the score function $\grad\ln p_{T-t}$ as $\vs_{T-t}$, and discretize SDE.~\ref{sde:rev_ou} as
\begin{equation*}
    \der \tilde{\rvx}_{t} = \left(\tilde{\rvx}_{t} + 2 s_{T-k\eta}(\tilde{\rvx}_{k\eta})\right) \der t + \sqrt{2}\der \mB_t\quad \mathrm{where}\quad t\in[k\eta, (k+1)\eta],
\end{equation*}
which actually is an OU process and has the following closed solution of $\tilde{\rvx}_{(k+1)h}$, i.e.,
\begin{equation*}
    \tilde{\rvx}_{(k+1)\eta} = e^\eta\cdot \tilde{\rvx}_{k\eta} - 2(1-e^\eta)\cdot s_{T-k\eta}(\tilde{\rvx}_{T-k\eta}) + \sqrt{e^{2\eta}-1} \cdot \xi\quad\mathrm{and}\quad \xi\sim \mathcal{N}(\vzero,\mI),
\end{equation*}
which matches the update in empirical work.
In the analysis of diffusion models~\cite{chen2022sampling}, we note that $\eta$ should be extremely small to control the discretization error, i.e.,
\begin{equation*}
\E\left[\int_{0}^\eta\left\|s_{T-k\eta}(\tilde{\rvx}_{k\eta}) - \grad\ln p_{T-(k\eta+\tau)}(\tilde{\rvx}_{T-(k\eta+\tau)})\right\|^2 \der \tau\right].
\end{equation*}
Since the step size $\eta$ should be small ($\Omega(\epsilon)$), there will be $T/\epsilon$ scores that need to be approximated, which causes a substantial computational cost.

The bottleneck of this type of algorithm is that they want to sample the target distribution by discretizing the reverse SDE.
In the following, I will introduce a method to sample with the reverse transition kernel, which can reduce the number of scores required to be estimated from $T/\epsilon$ to $T/L$ where $L$ denotes the uniformed smoothness of the log density of $p_t$.


%-------------Mar. 20---------------backup-------------
\begin{equation*}
    u(\vz_s) = \int_{\tilde{z}\in \mathcal{B}(\vz_s,r)
    \cap \mathcal{B}(\vzero,R)} \tilde{q}(\tilde{\vz}|{\vz_s})\der\tilde{\vz},
\end{equation*}
the transition kernel after Step~\ref{step:inball} will be denoted as 
\begin{equation}
    \label{eq:app_trans_ker_proj}
    q^\prime(\vz^\prime|\vz_s) = (1-u(\vz_s))\cdot \delta_{\vz_s}(\vz^\prime) + \tilde{q}(\vz^\prime|\vz_s)\cdot \vone\left[\vz^\prime\in  \mathcal{B}(\vz_s,r)
    \cap \mathcal{B}(\vzero,R) \right].
\end{equation}
Considering the 1/2-lazy version of the process, we have the transition distribution satisfies
\begin{equation}
    \label{eq:app_trans_ker_lazy}
    \mathcal{T}^\prime_{\vz_s}(\vz^\prime) = \frac{1}{2}\delta_{\vz_s}(\vz^\prime) + \frac{1}{2}q^\prime(\vz^\prime|\vz_s).
\end{equation}
In this condition, we define the accept rate which satisfies
\begin{equation*}
    a_{\vz_s}(\vz^\prime) = \min\left\{1, \frac{\mathcal{T}^\prime_{\vz^\prime}(\vz_s)}{\mathcal{T}^\prime_{\vz_s}(\vz^\prime)} \cdot \exp\left(-r_\theta(\vz_s, \vz^\prime)\right)\right\}\quad \mathrm{where}\quad a_{\vz_s}(\vz^\prime) = a(\vz^\prime - (\vz_s - \tau\cdot s_{\theta}(\vz_s)), \vz_s). 
\end{equation*}
Then, the transition kernel for the projected MALA implementation of Alg,~\ref{alg:inner_mala} will be 
\begin{equation*}
    \mathcal{T}_{\vz_s}(\vz_{s+1}) = \left(1-a_{\vz_s}(\vz_{s+1})\right)\cdot \delta_{\vz_s}(\vz_{s+1}) + a_{\vz_s}(\vz_{s+1})\cdot \mathcal{T}^\prime_{\vz_s}(\vz_{s+1}).
\end{equation*}


Suppose 
\begin{equation*}
    u_*(\vz_s) = \int_{\tilde{z}\in \mathcal{B}(\vz_s,r)
    \cap \mathcal{B}(\vzero,R)} \tilde{q}_*(\tilde{\vz}|{\vz_s})\der\tilde{\vz}, 
\end{equation*}
the transition kernel after Step~\ref{step:inball} will be denoted as 
\begin{equation*}
    q^\prime_*(\vz^\prime|\vz_s) = (1-u_*(\vz_s))\cdot \cdot \delta_{\vz_s}(\vz^\prime) + \tilde{q}_*(\vz^\prime|\vz_s)\cdot \vone\left[\vz^\prime\in  \mathcal{B}(\vz_s,r)
    \cap \mathcal{B}(\vzero,R) \right].   
\end{equation*}
Similar to the previous settings, we consider the 1/2-lazy version of the process, we have the transition distribution satisfies
\begin{equation*}
    \mathcal{T}^\prime_{*, \vz_s}(\vz^\prime) = \frac{1}{2}\delta_{\vz_s}(\vz^\prime) + \frac{1}{2}q_*^\prime(\vz^\prime|\vz_s).
\end{equation*}
In this condition, we define the accept rate which satisfies
\begin{equation*}
    a_{*, \vz_s}(\vz^\prime) = \min\left\{1, \frac{\mathcal{T}^\prime_{*, \vz^\prime}(\vz_s)}{\mathcal{T}^\prime_{*,\vz_s}(\vz^\prime)} \cdot \exp\left(-\left(g(\vz^\prime)-g(\vz_s)\right)\right)\right\}.
\end{equation*}
Then, the transition kernel for the accurate projected MALA will be 
\begin{equation*}
    \mathcal{T}_{*,\vz_s}(\vz_{s+1}) = \left(1-a_{*, \vz_s}(\vz_{s+1})\right)\cdot \delta_{\vz_s}(\vz_{s+1}) + a_{*,\vz_s}(\vz_{s+1})\cdot \mathcal{T}^\prime_{*, \vz_s}(\vz_{s+1}).
\end{equation*}
It is easy to verify that the Markov process of accurately projected MALA is time-reversible.
Besides,~\cite{zhang2017hitting} has shown that the unique stationary distribution of this process is
\begin{equation*}
    p_*(\vz|\vx_0)\propto \exp(-g(\vz))\cdot \vone\left(\vz\in\mathcal{B}(0,R)\right).
\end{equation*}


\begin{equation*}
        \begin{aligned}
            &\gT_{\vz}(\gA) = \int_{\gA} \gT_{\vz}(\vz^\prime)\der \vz^\prime  = \int_{\gA} a_z(\vz^\prime)\gT^\prime_{\vz}(\vz^\prime)\der \vz^\prime\\
            &\gT_{*,\vz}(\gA) = \int_{\gA} \gT_{*,\vz}(\vz^\prime)\der\vz^\prime = \int_{\gA} a_{*,\vz}(\vz^\prime)\gT^\prime_{*,\vz}(\vz^\prime)\der \vz^\prime.
        \end{aligned}
    \end{equation*}

\begin{equation}
        \label{eq:case_1_term21_refor}
        \begin{aligned}
            & \frac{\int_\gA \left(a_{\vz}(\vz^\prime) - a_{*,\vz}(\vz^\prime)\right) \gT^\prime_{\vz}(\vz^\prime) \der\vz^\prime}{\int_\gA a_{*,\vz}(\vz^\prime)\gT_{*,\vz}^\prime(\vz^\prime)\der\vz^\prime} =  \frac{\int_\gA \left(a_{\vz}(\vz^\prime) - a_{*,\vz}(\vz^\prime)\right) \gT^\prime_{\vz}(\vz^\prime) \der\vz^\prime}{\int_{\gA} a_{*,\vz}(\vz^\prime)\gT^\prime_{\vz}(\vz^\prime) \der \vz^\prime} \cdot \frac{\int_{\gA} a_{*,\vz}(\vz^\prime)\gT^\prime_{\vz}(\vz^\prime) \der \vz^\prime}{\int_\gA a_{*,\vz}(\vz^\prime)\gT_{*,\vz}^\prime(\vz^\prime)\der\vz^\prime}.
        \end{aligned}
    \end{equation}


%--------------------Another version----------------
\textcolor{blue}{\hrule}
\paragraph{Another version.}
In this version, we consider the implementation of Alg~\ref{alg:rtk} without projection, i.e., Step.~\ref{step:inball}.
According to Step~\ref{step:ula}, the transition distribution satisfies
\begin{equation*}
    \tilde{Q}_{\vz_s} = \mathcal{N}\left(\vz_s - \tau\cdot s_\theta(\vz_s), 2\tau\right)
\end{equation*}
with a density function
\begin{equation*}
    \tilde{q}(\tilde{\vz}_s|\vz_s) = \varphi_{2\tau}\left(\tilde{\vz}_s - \left(\vz_s - \tau\cdot \grad s_\theta(\vz_s)\right)\right).
\end{equation*}
Hence, a $1/2$-lazy version of the transition distribution becomes
\begin{equation*}
    \gT^\prime_{\vz_s}(\der\vz^\prime) = \frac{1}{2}\cdot \delta_{\vz_s}(\der\vz^\prime) + \frac{1}{2}\cdot \tilde{Q}_{\vz_s}(\der \vz^\prime).
\end{equation*}
Then, with the following Metropolis-Hastings filter,
\begin{equation*}
    a_{\vz_s}(\vz^\prime) = \min\left\{1, \frac{\tilde{q}(\vz_s|\vz^\prime)}{\tilde{q}(\vz^\prime|\vz_s)} \cdot \exp\left(-r_\theta( \vz^\prime,\vz_s)\right)\right\}\quad \mathrm{where}\quad a_{\vz_s}(\vz^\prime) = a(\vz^\prime - (\vz_s - \tau\cdot s_{\theta}(\vz_s)), \vz_s), 
\end{equation*}
the transition kernel for the projected MALA implementation of Alg,~\ref{alg:inner_mala} will be 
\begin{equation*}
    \gT_{\vz_s}(\der \vz_{s+1}) =  \gT^\prime_{\vz_s}(\der \vz_{s+1})\cdot a_{\vz_s}(\vz_{s+1})+\left(1- \int a_{\vz_s}(\vz^\prime) \gT^\prime_{\vz_s}(\der \vz^\prime)\right)\cdot \delta_{\vz_s}(\der\vz_{s+1}).
\end{equation*}

Next, we also calculate the standard projected MALA with the knowledge of accurate $g(\vz)-g(\vz^\prime)$ and $\grad g(\vz)$. 
In this condition, the ULA step will provide
\begin{equation*}
    \tilde{Q}_{*, \vz_s} = \mathcal{N}\left(\vz_s - \tau\cdot \grad g(\vz_s), 2\tau\right)
\end{equation*}
with a density function
\begin{equation*}
    \tilde{q}_*(\tilde{\vz}_s|\vz_s) = \varphi_{2\tau}\left(\tilde{\vz}_s - \left(\tau\cdot \grad g(\vz_s)\right)\right).
\end{equation*}
Hence, a $1/2$-lazy version of the transition distribution becomes
\begin{equation*}
    \gT^\prime_{*, \vz_s}(\der\vz^\prime) = \frac{1}{2}\cdot \delta_{\vz_s}(\der\vz^\prime) + \frac{1}{2}\cdot \tilde{Q}_{*,\vz_s}(\der \vz^\prime).
\end{equation*}
Then, with the following Metropolis-Hastings filter,
\begin{equation*}
    a_{*, \vz_s}(\vz^\prime) = \min\left\{1, \frac{\tilde{q}_*(\vz_s|\vz^\prime)}{\tilde{q}_*(\vz^\prime|\vz_s)} \cdot \exp\left(-\left(g(\vz^\prime)-g(\vz_s)\right)\right)\right\},
\end{equation*}
the transition kernel for the accurate projected MALA will be 
\begin{equation*}
    \gT_{*, \vz_s}(\der \vz_{s+1}) =  \gT^\prime_{*, \vz_s}(\der \vz_{s+1})\cdot a_{*, \vz_s}(\vz_{s+1})+\left(1- \int a_{*, \vz_s}(\vz^\prime) \gT^\prime_{*, \vz_s}(\der \vz^\prime)\right)\cdot \delta_{\vz_s}(\der\vz_{s+1}).
\end{equation*}
We will further show that the transition distribution of projected MALA implementation of Alg,~\ref{alg:inner_mala} can be $\delta$-close to the accurately projected MALA for some small quantity governed by $\tau$, which is provided in the following lemma.

We denote the underlying distribution of particles $\rvz_s$ as $\tilde{Q}_s$ with the transition kernel 
\begin{equation*}
    \tilde{Q}_{s+1|s}(\cdot|\vz) = \gT_{\vz}(\cdot),\quad \forall s\in\{0,1, \ldots, S-1\}.
\end{equation*}
Besides, we denote another underlying distribution of $\rvz_{*,s}$ as $\tilde{Q}_{*,s}$ with the transition kernel 
\begin{equation*}
    \tilde{Q}_{*, s+1|s}(\cdot|\vz) = \gT_{*, \vz}(\cdot),\quad \forall s\in\{0,1, \ldots, S-1\}.
\end{equation*}
In this condition, we have
\begin{equation*}
    \TVD{\tilde{Q}_S}{Q_*} = \TVD{\tilde{Q}_S}{\tilde{Q}_{*,S}} + \TVD{\tilde{Q}_{*,S}}{Q_*}
\end{equation*}
For the first term, it has
\begin{equation*}
    \begin{aligned}
        \TVD{\tilde{Q}_S}{\tilde{Q}_{*,S}} = & \TVD{\tilde{Q}_{*,S}}{\tilde{Q}_S} \le \sqrt{\frac{1}{2}\KL{\tilde{Q}_{*,S}}{\tilde{Q}_S}}\\
        = & \sqrt{\frac{1}{2}}\cdot \sqrt{\KL{\tilde{Q}_{*,S-1}}{\tilde{Q}_{S-1}} + \E_{\tilde{Q}_{*,S-1}}\left[\KL{\tilde{Q}_{*,S|S-1}(\cdot|\rvz)}{\tilde{Q}_{S|S-1}(\cdot|\rvz)}\right]}\\
        = & \sqrt{\frac{1}{2}}\cdot \sqrt{\KL{\tilde{Q}_{*,S-1}}{\tilde{Q}_{S-1}} + \E_{\tilde{Q}_{*,S-1}}\left[\KL{\gT_{*,\rvz}}{\gT_{\rvz}}\right]}\\
        = &\sqrt{\frac{1}{2}}\cdot \sqrt{\sum_{s=1}^{S}\E_{\tilde{Q}_{*,s-1}}\left[\KL{\gT_{*,\rvz}}{\gT_{\rvz}}\right]}
    \end{aligned}
\end{equation*}
where the first inequality follows from the chain rule of TVD shown in Lemma~\ref{lem:tv_chain_rule} and the last inequality follows from recursion.
In this condition, we have
\begin{equation*}
    \KL{\gT_{*,\vz}}{\gT_{\vz}} \le  \int_{\R^d - \{\vz\}} \ln \frac{\gT_{*,\vz}(\der \vz^\prime)}{\gT_{\vz}(\der \vz^\prime)} \cdot \gT_{*,\vz}(\der \vz^\prime) + \ln \frac{\gT_{*,\vz}(\der \vz)}{\gT_{\vz}(\der \vz)} \cdot \gT_{*,\vz}(\der \vz)
\end{equation*}
For the first term, we have
\begin{equation*}
    \begin{aligned}
        & \int_{\R^d - \{\vz\}} \ln \frac{\gT_{*,\vz}(\der \vz^\prime)}{\gT_{\vz}(\der \vz^\prime)} \cdot \gT_{*,\vz}(\der \vz^\prime)\\
        & = \int_{\R^d - \{\vz\}} \ln\frac{\gT^\prime_{*, \vz}(\der \vz^\prime)\cdot a_{*, \vz}(\vz^\prime)}{\gT^\prime_{\vz}(\der \vz^\prime)\cdot a_{\vz}(\vz^\prime)}\cdot \gT^\prime_{*, \vz}(\der \vz^\prime)\cdot a_{*, \vz}(\vz^\prime)\\
        & = \int_{\R^d - \{\vz\}} \ln \frac{\tilde{Q}_{*,\vz}(\der\vz^\prime)\cdot a_{*,\vz}(vz^\prime)}{\tilde{Q}_{\vz}(\der\vz^\prime)\cdot a_{\vz}(\vz^\prime)}\cdot \frac{1}{2}\cdot \tilde{Q}_{*,\vz}(\der\vz^\prime)\cdot a_{*,\vz}(vz^\prime)\\
        & = \frac{1}{2}\cdot \int_{\R^d - \{\vz\}} \ln \frac{\tilde{q}_*(\vz^\prime|\vz)\cdot a_{*,\vz}(\vz^\prime)}{\tilde{q}(\vz^\prime|\vz)\cdot a_{\vz}(\vz^\prime)}\cdot \tilde{q}_*(\vz^\prime|\vz)\cdot a_{*,\vz}(\vz^\prime)\der\vz^\prime
    \end{aligned}
\end{equation*}

%----------Apr. 23 backup

\begin{corollary}
    \label{cor:inner_convergence}
    Under Assumption~\ref{ass:lips_score}--\ref{ass:second_moment}, for any $\epsilon\in(0,1)$, let $\tilde{\mu}_*(\vz)\propto \exp(-g(\vz))\vone[\vz\in\mathcal{B}(\vzero,R)]$ be the truncated target distribution in $\mathcal{B}(\vzero,R)$ with $R = \tilde{\mathcal{O}} \left((d+m_2^2 + \|\vx_0\|^2)^{1/2}\right)$.
    Suppose $\tilde{\mu}_0(\{\|\rvx\|\ge R/2\})\le \epsilon/16$, the step size $\tau=\tilde{\mathcal{O}}((d+m_2^2+\|\vx_0\|^2)^{-1}\cdot L^{-2})$ and the score estimation error satisfies $\epsilon_{\mathrm{score}} = \tilde{\mathcal{O}}(\epsilon\cdot (d+m_2^2+\|\vx_0\|^2)^{-1})$, then for any $\lambda$-warm start with respect to $\tilde{\mu}_*$ the output of both standard and projected implementation of Alg.~\ref{alg:inner_mala} satisfies
    \begin{equation*}
        \TVD{\mu_S}{\mu_*} \le \frac{3\epsilon}{4} +  \lambda \left(1- L^2\tau^2\right)^S.
    \end{equation*}
\end{corollary}
\begin{proof}
    Since we provide the lower bound of the Cheeger constant $\rho$ of $\tilde{\mu}_*$, we introduce such a lower bound, i.e., $\rho\ge \pi/(16R)$, to Theorem~\ref{thm:inner_convergence} to make the bound more explicit.
    We should first note that the Cheeger constant will not affect the choice of $R$ and the step size $\tau$.
    On the other hand, it will make the score estimation error satisfy
    \begin{equation*}
        \epsilon_{\mathrm{score}}\le C_{\mathrm{score}} \cdot \frac{\rho\epsilon}{\sqrt{d\log\frac{8S}{\epsilon}}}\le C_{\mathrm{score}}^\prime \cdot \frac{\epsilon}{\sqrt{d(d+m_2^2+\|\vx_0\|^2)}}\cdot \left(\log\frac{16S}{\epsilon}\right)^{-1} = \tilde{\mathcal{O}}\left(\frac{\epsilon}{d+m_2^2+\|\vx_0\|^2}\right)
    \end{equation*}
    where $C_{\mathrm{score}}^\prime = C_{\mathrm{score}} \pi/(16\cdot 63)$.
    Besides, the convergence rate will become
    \begin{equation*}
        \TVD{\mu_S}{\mu_*} \le \frac{3\epsilon}{4} +  \left(1- \frac{C_0^\prime\tau}{(d+m_2^2 + \|\vx_0\|^2)\log \frac{16S}{\epsilon}} \right)^S \approx \frac{3\epsilon}{4} + \left(1-L^2\tau^2\right)^S
    \end{equation*}
    since it has
    \begin{equation*}
        \rho^2 \ge \frac{\pi^2}{16^2 R^2} = \left(\frac{\pi}{16\cdot 63}\right)^2 \cdot \left(d+m_2^2+\|\vx_0\|^2\right) \cdot \left(\log \frac{16S}{\epsilon}\right) = \mathcal{O}(\tau^{-1} L^{-2}).
    \end{equation*}
    Hence, the proof is completed.
\end{proof}

\begin{definition}[Poincar\'e inequality definition]
    The Markov process is said to satisfy a Poincar\'e inequality (PI) with constant $C_{\mathrm{PI}}$ if for all functions $f\in L^2(\pi)$, 
    \begin{equation*}
        \int f(-\gL)f\der\mu \ge C^{-1}_{\mathrm{PI}} \cdot \mathrm{Var}_\mu\left(f\right)
    \end{equation*}
\end{definition}

\begin{remark}[Example 1.2.21 in~\cite{sinho2024logconcave}]
    For the Langevin diffusion, the Poincar\'e inequality reads
    \begin{equation*}
        \mathrm{Var}_\mu f\le C_{\mathrm{PI}}\E_{\mu}\left[\left\|\grad f\right\|^2\right]
    \end{equation*}
    for all function $f\colon \R^d\rightarrow \R$.
\end{remark}

\begin{definition}[Definition 2.5.16 in~\cite{sinho2024logconcave}]
    For $p,q\in [1,\infty]$ with $q\ge p$, the $L^p-L^q$ Poincar\'e inequality of the distribution $\mu$ asserts that for all smooth $f\colon \R^d\rightarrow \R$, i.e., 
    \begin{equation*}
        \left\|f - \E_{\mu}[f]\right\|_{L^p(\mu)} \le C_{p,q}\left\| \left\|\grad f\right\| \right\|_{L^q(\mu)}
    \end{equation*}
\end{definition}



\begin{proposition}[\cite{milman2009role}]
    \label{prop:milman2009}
    Suppose $p,q,\hat{p},\hat{q} \in [1,\infty]$ are such that $p\le \hat{p}$ and $q\le \hat{q}$ and $p^{-1}- q^{-1} = \hat{p}^{-1} - \hat{q}^{-1}$. Then
    \begin{equation*}
        C_{\hat{p},\hat{q}}\le \hat{p}/ p \cdot C_{p,q}.
    \end{equation*}
\end{proposition}


\begin{remark}
    \label{def:relation_pi_chee}
    In $L^p-L^q$ Poincar\'e inequality, the usual Poincar\'e inequality is $L^2-L^2$ Poincar\'e inequality with $C_{2,2} = \sqrt{C_{\mathrm{PI}}}$, whereas Eq.~\ref{ineq:cheeger_inequality} is an $L^1-L^1$ Poincar\'e inequality with $C_{1,1} = 2\mathrm{Ch}$.
    Combining with Proposition~\ref{prop:milman2009}, we have
    \begin{equation*}
        \begin{aligned}
            2\mathrm{Ch} = C_{1,1} \ge \frac{1}{2}\cdot C_{2,2} = \frac{\sqrt{C_{\mathrm{PI}}}}{2}\quad\Leftrightarrow\quad \mathrm{Ch}\ge \frac{\sqrt{C_{\mathrm{PI}}}}{4}.
        \end{aligned}
    \end{equation*}
\end{remark}

\begin{lemma}[Theorem 24 in~\cite{lee2018kannan}]
    \label{lem:thm22_lee2018kannan}
    For any log-concave density $p$ in $\R^d$ with covariance matrix $\mA$ the Cheeger constant satisfies
    \begin{equation*}
        TBC
    \end{equation*}
\end{lemma}

\begin{corollary}
    \label{cor:truncted_che_constant}
    Suppose $\Omega = \mathcal{B}(\vzero,R)$ in Eq.~\ref{def:sta_tilde_mu_*}, the Cheeger constant of $\tilde{\mu}_*$ satisfies $\mathrm{Ch}\ge \pi/16R$.
\end{corollary}
\begin{proof}
    Combining the definition of $\tilde{\mu}_*$ in Eq.~\ref{def:sta_tilde_mu_*} and Lemma~\ref{lem:thm22_lee2018kannan}, we know the Poincar\'e constant of $\tilde{\mu}_*$ satisfies $C_{\mathrm{PI}} = \pi^2/(4\cdot (2R)^2)$.
    Then, we introduce Remark~\ref{def:relation_pi_chee}, and have the Cheeger constant of $\tilde{\mu}_*$ satisfies
    \begin{equation*}
        \mathrm{Ch}\ge \frac{\sqrt{C_{\mathrm{PI}}}}{4} = \frac{\pi}{16R}.
    \end{equation*}
    Hence, the proof is completed.
\end{proof}


%============== May. 14th ===============

In this condition, for any two timestamps 
$t^\prime>t$, it has
\begin{equation}
    \label{ineq:rev_tk}
    p_{t|t^\prime}(\vx|\vx^\prime) = \frac{p_t(\vx)\cdot p_{t^\prime|t}(\vx^\prime|\vx)}{p_{t^\prime}(\vx^\prime)} \propto \exp\left(-f_t(\vx)-\frac{\left\|\vx^\prime - \vx\cdot 
 e^{-(t^\prime-t)}\right\|^2}{2(1-e^{-2(t^\prime-t)})}\right),
\end{equation}
which can be proved by Lemma~\ref{lem:rev_trans_ker_form}.

Then, for the process $\{\rbkwx_k\}$, we define the particle $\rbkwx_k = \rvx_{(K-k)\eta}$, which means it is initialized with $\rbkwx\sim p_{K\eta}$ and has the following transition kernel
\begin{equation}
    \label{ineq:rev_tk_app}
    \begin{aligned}
        \bkwp_{k+1|k}(\vx^\prime|\vx) &= \bkwp_{k|k+1}(\vx|\vx^\prime)\cdot \bkwp_{k+1}(\vx^\prime)\big/{\bkwp_{k}(\vx)} = p_{T-k\eta|T-(k+1)\eta}(\vx|\vx^\prime)\cdot p_{T-(k+1)\eta}(\vx^\prime)\big/{p_{T-k\eta}(\vx)}\\
        & = p_{T-(k+1)\eta|T-k\eta} (\vx^\prime|\vx)\propto \exp\left(-f_{T-(k+1)\eta}(\vx^\prime)-\frac{\left\|\vx - \vx^\prime\cdot e^{-\eta}\right\|^2}{2(1-e^{-2\eta})}\right).
    \end{aligned}
\end{equation}


In this condition, we can fast obtain samples whose underlying distribution approximates $p_{t|t^\prime}(\vx|\vx^\prime)$ by requiring
\begin{equation*}
    - \grad^2 \ln \bkwp_{k+1|k}(\vx|\vx^\prime) = \grad^2 f_{T-(k+1)\eta}(\vx) +  \frac{e^{-2\eta}}{1-e^{-2\eta}}\cdot \mI \succeq c\cdot \mI,
\end{equation*}
which only requires $\eta$ to be a constant level with respect to the smoothness of $f_{(K-k-1)\eta}(\vx)$.
\begin{align}
    & \TVD{\hat{p}_{k+1|k}(\cdot|\vx)}{p_{(K-k-1)\eta|(K-k)\eta}(\cdot|\vx)} \le \delta_k,\label{ineq:tvd_appro}\tag{TV Approximation}\\
    & \KL{\hat{p}_{k+1|k}(\cdot|\vx)}{p_{(K-k-1)\eta|(K-k)\eta}(\cdot|\vx)} \le \delta_k. \label{ineq:kld_appro}\tag{KL Approximation}
\end{align}


All these assumptions are required in~\cite{chen2022sampling}.
\begin{remark}
    \cite{chen2023improved} shows that Assumption~\ref{ass:lips_score} can be removed via early stopping, at the cost of polynomially larger iteration complexity. The idea is that if $p_*$ has compact support but does not necessarily satisfy Assumption~\ref{ass:lips_score} then $p_\delta$ will satisfy Assumption~\ref{ass:lips_score} if $\delta>0$. 
     By applying our analysis up to time $T-\delta$ instead of time $T$ one can show that a suitable projection of the output distribution is close in Wasserstein distance to $p_*$. 
     For brevity, we do not consider this extension of our
    results here.
\end{remark}
